# Supplementary material for: Composable computation in discrete chemical reaction networks
Source: arXiv:1903.02637 source file (2019-06-01)
Supplement: Supplementary file 1 [file appendix.tex]

\newpage
\appendix

\noindent{\LARGE{\bf Appendix}}

\vspace{0.5cm}

\noindent
\opt{sub}{This appendix contains proofs and intermediate technical lemmas not given in detail in the main paper.}

\opt{sub}{
    \section{Composability and oblivious CRNs}
    \label{sec:appendix-composability}
    \input{sections/composability-and-oblivious}

    \section{One-dimensional case}
    \label{sec:appendix-1d-case}
    \restateThmOneDimMC
    \proofThmOneDimMC
    
    \subsection{1D Leaderless Case}
    \label{sec:leaderless-1D}
    \input{sections/leaderless}

    \section{Contradiction lemma}
    \label{sec:appendix-contradiction-lemma}
    \restateLemDicksonContradiction
    \proofLemDicksonContradiction

    \section{Construction}
    \label{sec:appendix-construction}
    \lemAndProofQuiltAffineConstruction
    
    \restateLemGeneralConstruction
    \proofLemGeneralConstruction

    \section{Output-oblivious functions are eventually min of quilt-affine functions}
    \input{sections/full-dim-sunshine}
    \input{sections/full-dim-determined-regions}
    \input{sections/full-dim-underdetermined-regions}
}

\opt{full}{
    \section{1D Leaderless Case}
    \label{sec:leaderless-1D}
    \input{sections/leaderless}
}

\opt{sub}{\input{sections/continuous-compare}}
